# Supplementary material for: Transferring to Real-World Layouts: A Depth-aware Framework for Scene Adaptation
Source: arXiv:2311.12682 source file (2024-07-31)
Supplement: Supplementary file 1 [file appendix.tex]

\section*{Appendix}
\setcounter{section}{0}

\section{More Quantitative Results}

%\textbf{Transfer learning from University-1652 to small datasets.} 
%We evaluate the generalization ability of the baseline model on two small datasets, \ie, Oxford \cite{philbin2007object} and Pairs \cite{philbin2008lost}. Oxford and Pairs are two popular place recognition datasets. We directly evaluate our model on these two datasets without finetuning. Further, we also report the results on the revised Oxford and Paris datasets (denoted as ROxf and RPar) \cite{RITAC18}. In contrast to the generic feature trained on ImageNet \cite{deng2009imagenet}, the learned feature on University-1652 shows better generalization ability. Specifically, we try two different branches, \ie, $\mathcal{F}_s$ and $\mathcal{F}_g$, to extract features. $\mathcal{F}_s$ and $\mathcal{F}_g$ share the high-level feature space but pay attention to different low-level patterns of inputs from different platforms. $\mathcal{F}_s$ is learned on the satellite-view images and drone-view images, while $\mathcal{F}_g$ learns from ground-view images. As shown in Table \ref{table:loss}, $\mathcal{F}_g$ has achieved better performance than $\mathcal{F}_s$. We speculate that there are two main reasons. First, the test data in Oxford and Pairs are collected from Flickr, which is closer to the Google Street View images and the images retrieved from Google Image in the ground-view data. Second, $\mathcal{F}_s$ pay more attention to the vertical viewpoint changes instead of the horizontal viewpoint changes, which are common in Oxford and Paris.

\textbf{With/without Google Image data.} In the University-1652 training data, we introduce the ground-view images collected from Google Image. We observe that although the extra data retrieved from Google Image contains noise, most images are true-matched images of the target building. In Table \ref{table:Google}, we report the results with/without the Google Image training data. The baseline model trained with extra data generally boosts the performance not only on the ground-related tasks, \ie, Ground $\rightarrow$ Satellite and Satellite $\rightarrow$ Ground,  but on the drone-related tasks, \ie, Drone $\rightarrow$ Satellite and Satellite $\rightarrow$ Drone. The result also verifies that our baseline method could perform well against the noisy data in the training set.

\section{More Qualitative Results}
\textbf{Visualization of cross-view features.} 
We sample $500$ pairs of drone-view and satellite-view images in the test set to extract features and then apply the widely-used t-SNE \cite{van2014accelerating} to learn the 2D projection of every feature. As shown in Figure~\ref{fig:cluster}, the features of the same location are close, and the features of different target buildings are far away. It demonstrates that our baseline model learns the effective feature space, which is discriminative.

\section{More Details of University-1652}

\textbf{Building name list.} We show the name of the first $100$ buildings in University-1652 (see Table \ref{table:BuildingName}). 

\noindent\textbf{Data License.} We carefully check the data license from Google. There are two main points.
First, the data of Google Map and Google Earth could be used based on fair usage. We will follow the guideline on this official website \footnote{\url{https://www.google.com/permissions/geoguidelines/}}.
Second, several existing datasets have utilized the Google data. In practice, we will adopt a similar policy of existing datasets \footnote{\url{http://www.ok.ctrl.titech.ac.jp/~torii/project/247/}}$^,$ 
\footnote{\url{http://cs.uky.edu/~jacobs/datasets/cvusa/}} to release the dataset based on the academic request. 

\noindent\textbf{Frame-level metadata.} Besides drone-view videos, we also record the frame-level metadata, including the building name, longitude, latitude, altitude, heading, tilt and range (see Figure~\ref{fig:metadata}). Exploiting metadata is out of the scope of this paper, so we do not explore the usage of attributes in this work. But we think that the metadata could enable the future study, \eg, orientation alignment between drone-view images and satellite-view images. In the future, we will continue to study this problem.

%\noindent\textbf{Image samples.} We sample the images from three platforms in University-1652, and show them in Figure~\ref{fig:drone-data}, Figure~\ref{fig:satellite-data}, Figure~\ref{fig:ground-data}, and Figure~\ref{fig:google-data}, separately. Figure~\ref{fig:drone-data} shows drone-view images in University-1652, and Figure~\ref{fig:satellite-data} contains samples from the satellite-view data. Figure~\ref{fig:ground-data} displays the ground-view images collected from Google Street View, followed by the noisy training data that we obtained from the image search engine, \ie, Google Image.

%\textbf{Ground to Drone.}

%\textbf{Handcrafted Features.} Here we provide the results with the traditional handcrafted features, \ie, SIFT and SURF. 
\begin{figure*}[t]
\begin{center}
    \includegraphics[width=0.95\linewidth]{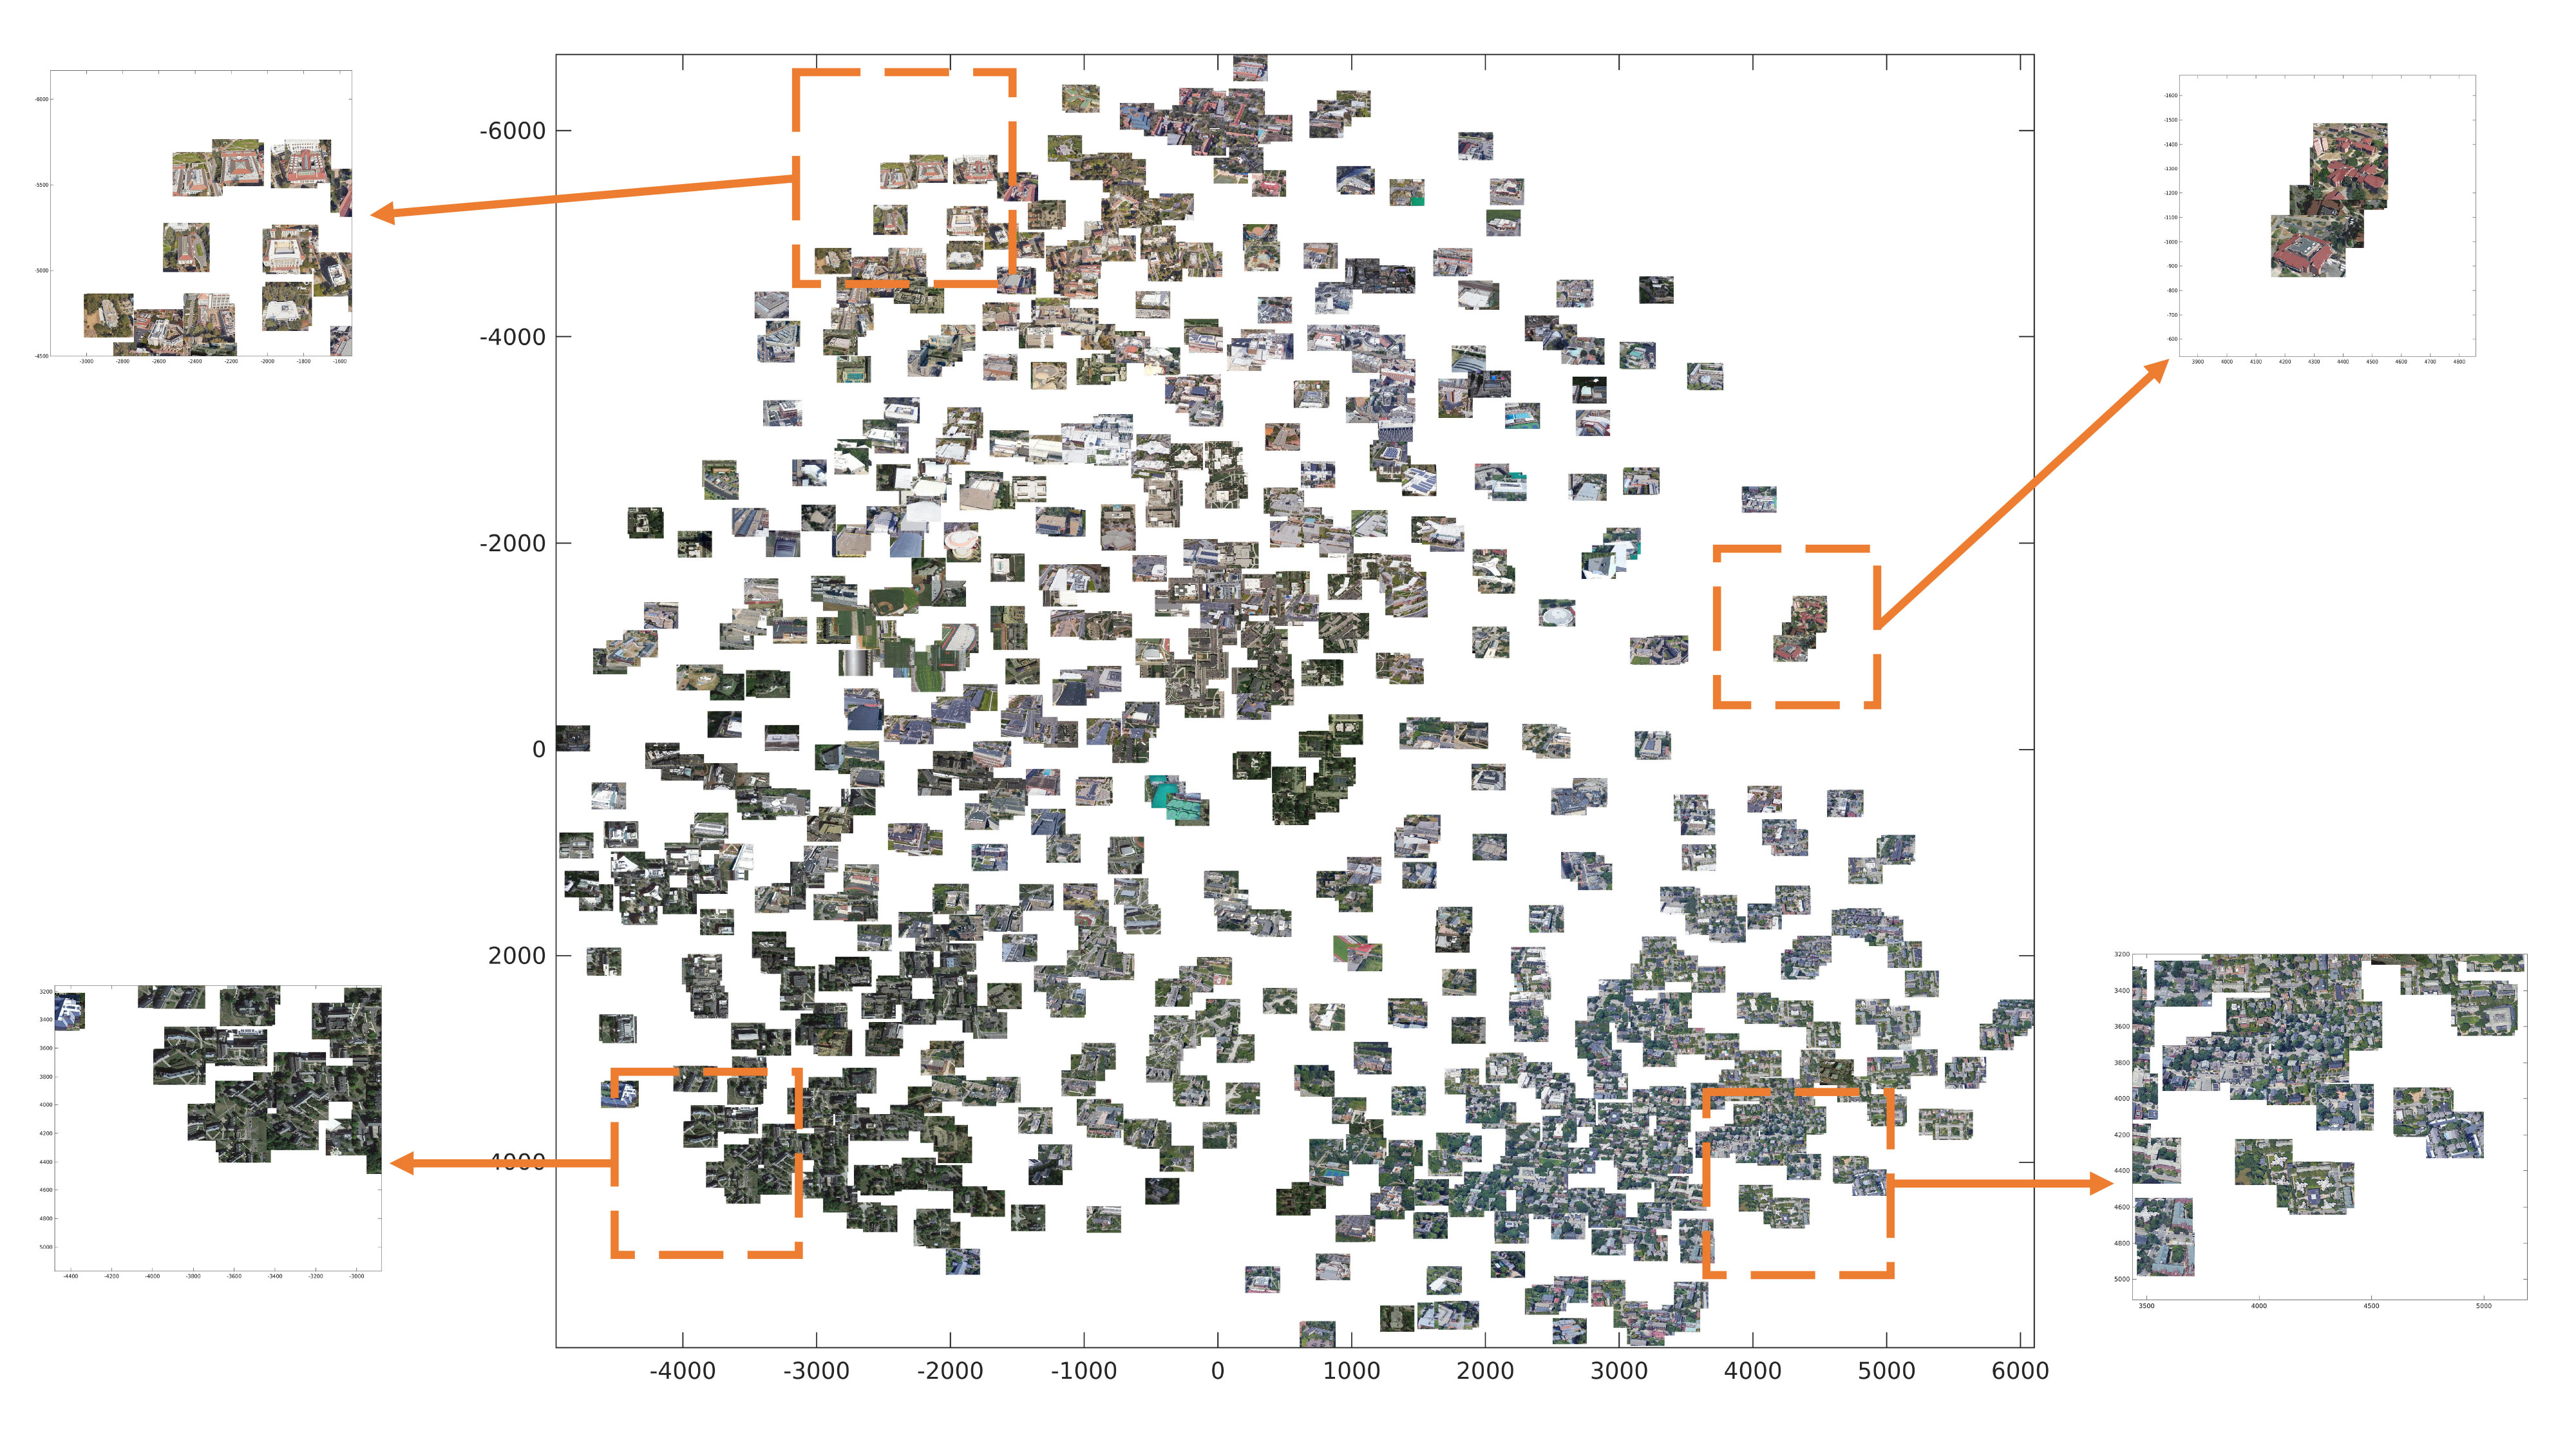}
\end{center}
%\vspace{-.2in}
     \caption{Visualization of cross-view features using t-SNE \cite{van2014accelerating} on University-1652. (Best viewed when zoomed in.)
     }\label{fig:cluster}
%\vspace{.3in}
\end{figure*}

\begin{figure}[t]
\begin{center}
    \includegraphics[width=1\linewidth]{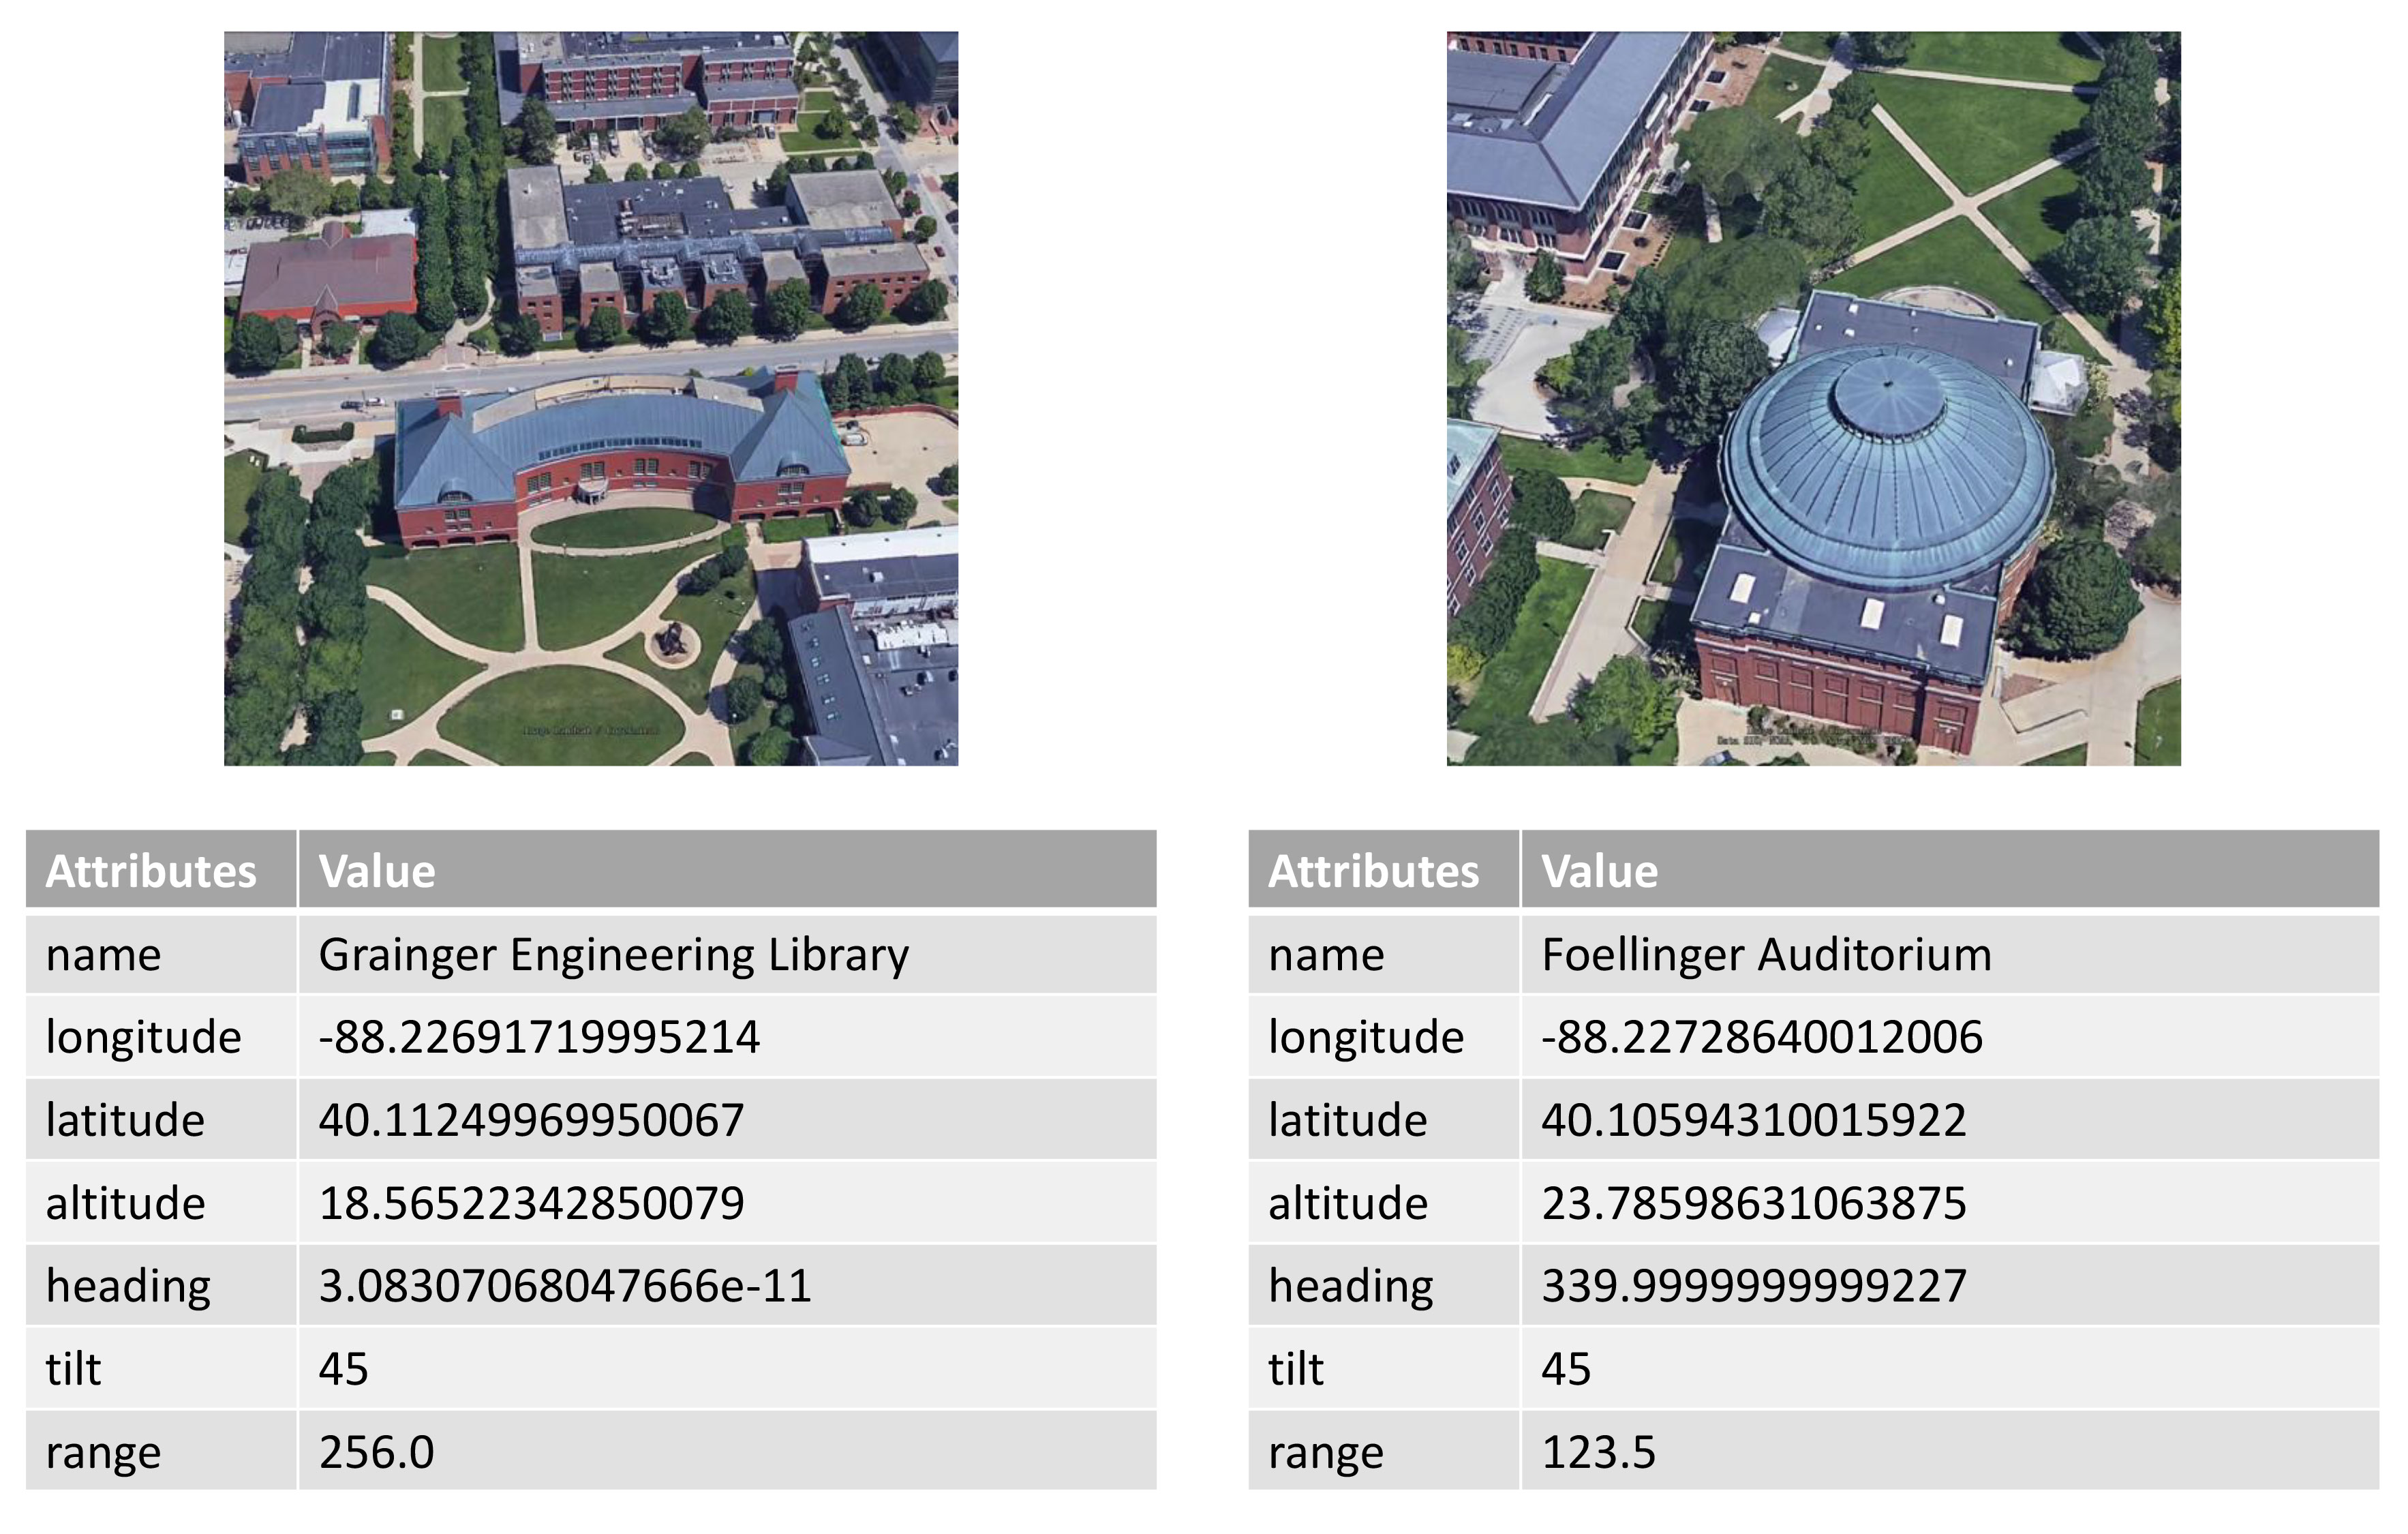}
\end{center}
%\vspace{-.2in}
     \caption{Metadata samples. We record attributes for every frame, including the building name, longitude, latitude, altitude, heading, tilt and range. }\label{fig:metadata}
\end{figure}

\setlength{\tabcolsep}{7pt}
\begin{table*}
\small
\begin{center}
\begin{tabular}{l|ccc|ccc|ccc|ccc}
\hline
\multirow{2}{*}{Model} & \multicolumn{3}{c|}{Drone $\rightarrow$ Satellite} & \multicolumn{3}{c|}{Satellite $\rightarrow$ Drone} & \multicolumn{3}{c|}{Ground $\rightarrow$ Satellite} & 
\multicolumn{3}{c}{Satellite $\rightarrow$ Ground}\\
  & R@1 & R@10 & AP & R@1 & R@10 & AP & R@1 & R@10 & AP & R@1 & R@10 & AP \\
\shline
Without noisy data  & 57.52 & 83.89 & 62.29 & 69.19 & 82.31 & 56.15 & \textbf{1.28} & 6.20 & 2.29& \textbf{1.57} & 7.13 & \textbf{1.52}\\
With noisy data & \textbf{58.49} & \textbf{85.23} &  \textbf{63.13} & \textbf{71.18} & \textbf{82.31} & \textbf{58.74} & 1.20 & \textbf{7.56} & \textbf{2.52} & 1.14 & \textbf{8.56} & 1.41 \\
\hline
\end{tabular}
\end{center}
%\vspace{-.2in}
\caption{Ablation study. With / without noisy training data from Google Image. The baseline model trained with the Google Image data is generally better in all four tasks. The result also verifies that our baseline method could perform well against the noise in the dataset.
}
\label{table:Google}
\end{table*}

%\newlength\savewidth\newcommand\shline{\noalign{\global\savewidth\arrayrulewidth
%  \global\arrayrulewidth 1pt}\hline\noalign{\global\arrayrulewidth\savewidth}}
  
\setlength{\tabcolsep}{1pt}
\begin{table*}
%\footnotesize
\small
\begin{center}
\begin{tabular}{c|c}
\hline
\multicolumn{2}{c}{Building Names}\\
\shline
Bibliothèque Saint-Jean, University of Alberta & Clare Drake Arena\\
Foote Field & Myer Horowitz Theatre\\
National Institute for Nanotechnology & St Joseph's College, Edmonton\\
Stollery Children's Hospital & Universiade Pavilion, University of Alberta\\
University of Alberta Hospital & Alberta B. Farrington Softball Stadium\\
Decision Theater, University of Alberta & Gammage Memorial Auditorium\\
Harrington–Birchett House & Industrial Arts Building\\
Irish Field & Louise Lincoln Kerr House and Studio\\
Matthews Hall, University of Alberta & Mona Plummer Aquatic Center\\
Old Main (Arizona State University) & Packard Stadium, University of Alberta\\
Security Building (Phoenix, Arizona) & Sun Devil Gym, University of Alberta\\
Sun Devil Stadium, University of Alberta & United States Post Office (Phoenix, Arizona)\\
Wells Fargo Arena (Tempe, Arizona) & Administration Building, University of Alberta\\
Wheeler Hall, University of Alberta & Marting Hall, University of Alberta\\
Malicky Center, University of Alberta & Burrell Memorial Observatory\\
Kleist Center for Art and Drama & Wilker Hall, University of Alberta\\
Kamm Hall, University of Alberta & Dietsch Hall, University of Alberta\\
Telfer Hall, University of Alberta & Ward Hall, University of Alberta\\
Thomas Center for Innovation and Growth (CIG) & Kulas Musical Arts Building, Baldwin Wallace University\\
Boesel Musical Arts Center, Baldwin Wallace University & Merner-Pfeiffer Hall, Baldwin Wallace University\\
Ritter Library, Baldwin Wallace University & Lindsay-Crossman Chapel, Baldwin Wallace University\\
Presidents House, Baldwin Wallace University & Student Activities Center (SAC), Baldwin Wallace University\\
Strosacker Hall (Union), Baldwin Wallace University & Bonds Hall, Baldwin Wallace University\\
Durst Welcome Center, Baldwin Wallace University & Lou Higgins Center, Baldwin Wallace University\\
Tressel Field @ Finnie Stadium, Baldwin Wallace University & Rutherford Library\\
Rudolph Ursprung Gymnasium, Baldwin Wallace University & Packard Athletic Center (formerly Bagley Hall), Baldwin Wallace University\\
Baldwin-Wallace College North Campus Historic District & Baldwin-Wallace College South Campus Historic District\\
Binghamton University Events Center, Binghamton University & Commonwealth Avenue, Boston University\\
Boston University Photonics Center, Boston University & Boston University School of Law, Boston University\\
Boston University Track and Tennis Center, Boston University & Boston University West Campus\\
BU Castle, Boston University & George Sherman Union, Boston University\\
John Hancock Student Village, Boston University & Marsh Chapel, Boston University\\
Metcalf Center for Science and Engineering, Boston University & Morse Auditorium, Boston University\\
Mugar Memorial Library, Boston University & Myles Standish Hall, Boston University\\
Questrom School of Business, Boston University & Shelton Hall (Boston University), Boston University\\
Walter Brown Arena, Boston University & Warren Towers, Boston University\\
Benson (Ezra Taft) Building, Brigham Young University & Brimhall (George H.) Building, Brigham Young University\\
BYU Conference Center, Brigham Young University & Centennial Carillon Tower, Brigham Young University\\
Chemicals Management Building, Brigham Young University & Clark (Herald R.) Building, Brigham Young University\\
Clark (J. Reuben) Building (Law School), Brigham Young University & Clyde (W.W.) Engineering Building, Brigham Young University\\
Crabtree (Roland A.) Technology Building, Brigham Young University & Eyring (Carl F.) Science Center, Brigham Young University\\
Faculty Office Building, Brigham Young University & Former Presidents' Home, Brigham Young University\\
BYU Testing Center, Grant (Heber J.) Building, Brigham Young University & Harman (Caroline Hemenway) Building, Brigham Young University\\
Harris (Franklin S.) Fine Arts Center, Brigham Young University & Kimball (Spencer W.) Tower, Brigham Young University\\
Knight (Amanda) Hall, Brigham Young University & Knight (Jesse) Building, Brigham Young University\\
Lee (Harold B.) Library, Brigham Young University & Life Sciences Building, Brigham Young University\\
Maeser (Karl G.) Building, Brigham Young University & Martin (Thomas L.) Building, Brigham Young University\\
McKay (David O.) Building, Brigham Young University & Smith (Joseph F.) Building, Brigham Young University\\
Smith (Joseph) Building, Brigham Young University & Snell (William H.) Building, Brigham Young University\\
Talmage (James E.) Math Sciences/Computer Building, Brigham Young University & Tanner (N. Eldon) Building, Brigham Young University\\
\hline
\end{tabular}
\end{center}
%\vspace{-.2in}
\caption{Due to the space limitation, here we show the first $100$ building names in the University-1652 dataset.
}
\label{table:BuildingName}
\end{table*}

\begin{comment}
\begin{figure*}[t]
\begin{center}
    \includegraphics[width=0.95\linewidth]{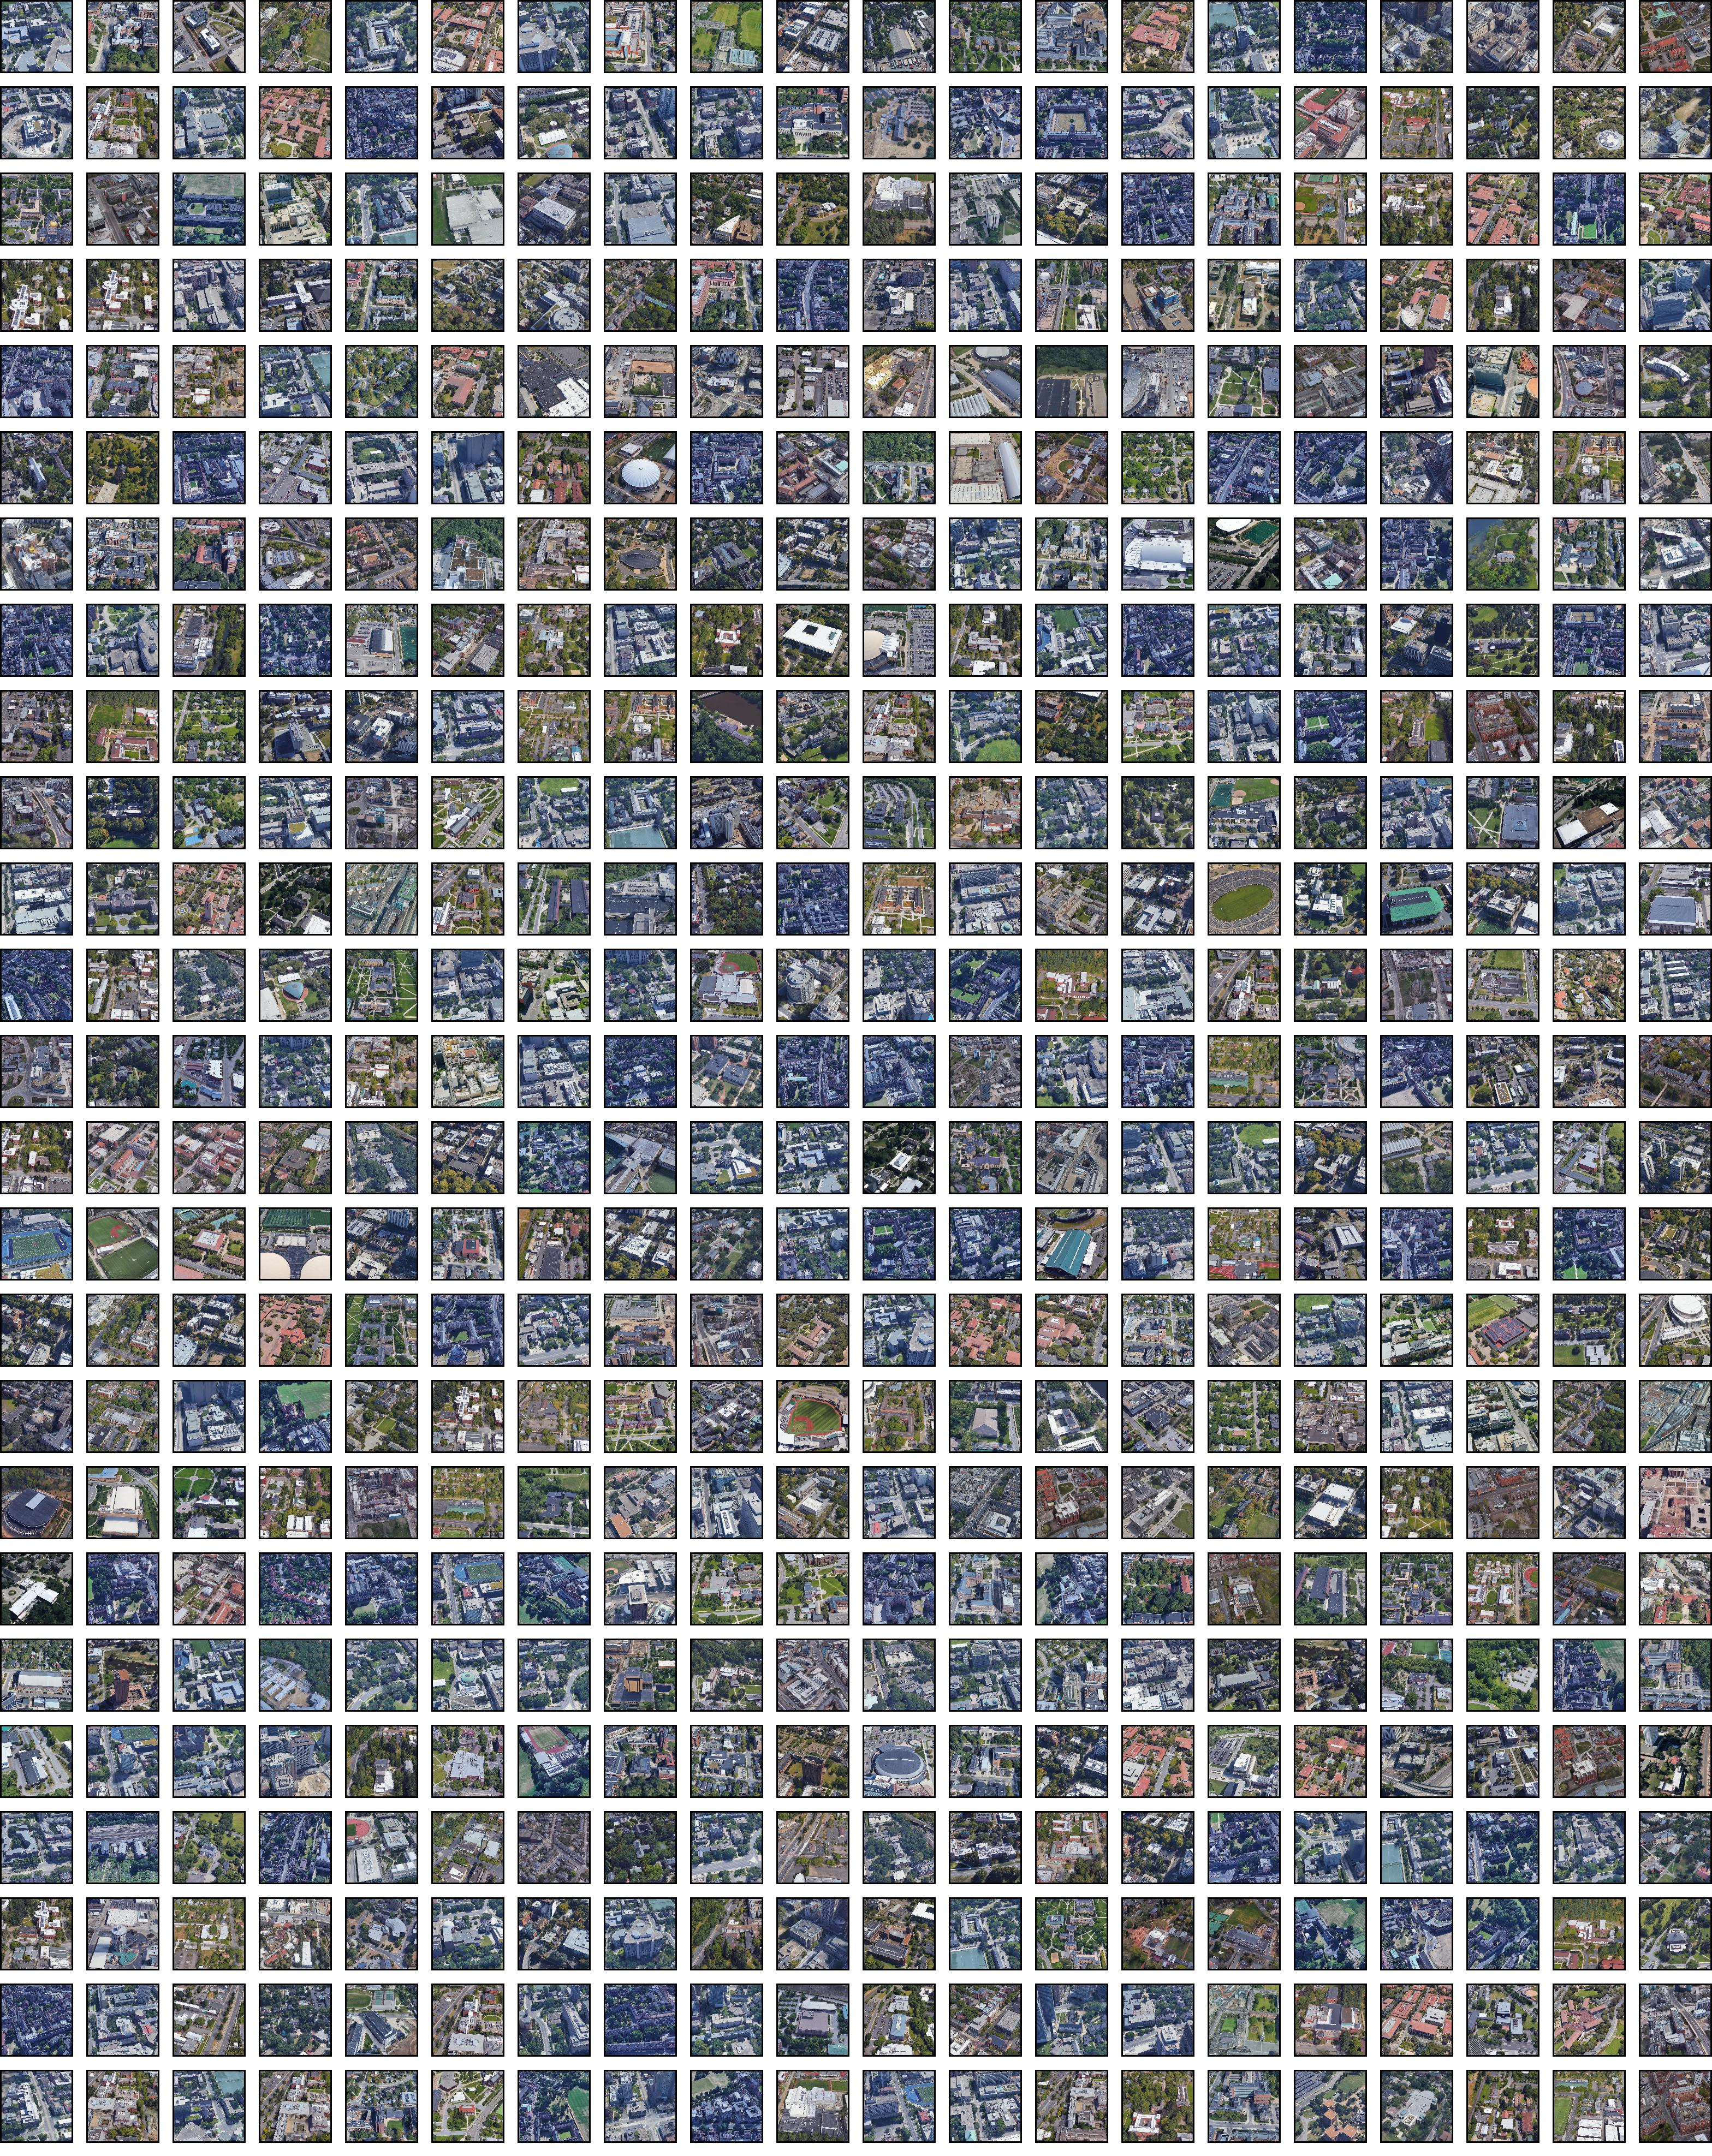}
\end{center}
%\vspace{-.25in}
     \caption{Images sampled from drone-view images of the University-1652 dataset.
     }\label{fig:drone-data}
\end{figure*}

\begin{figure*}[t]
\begin{center}
    \includegraphics[width=0.95\linewidth]{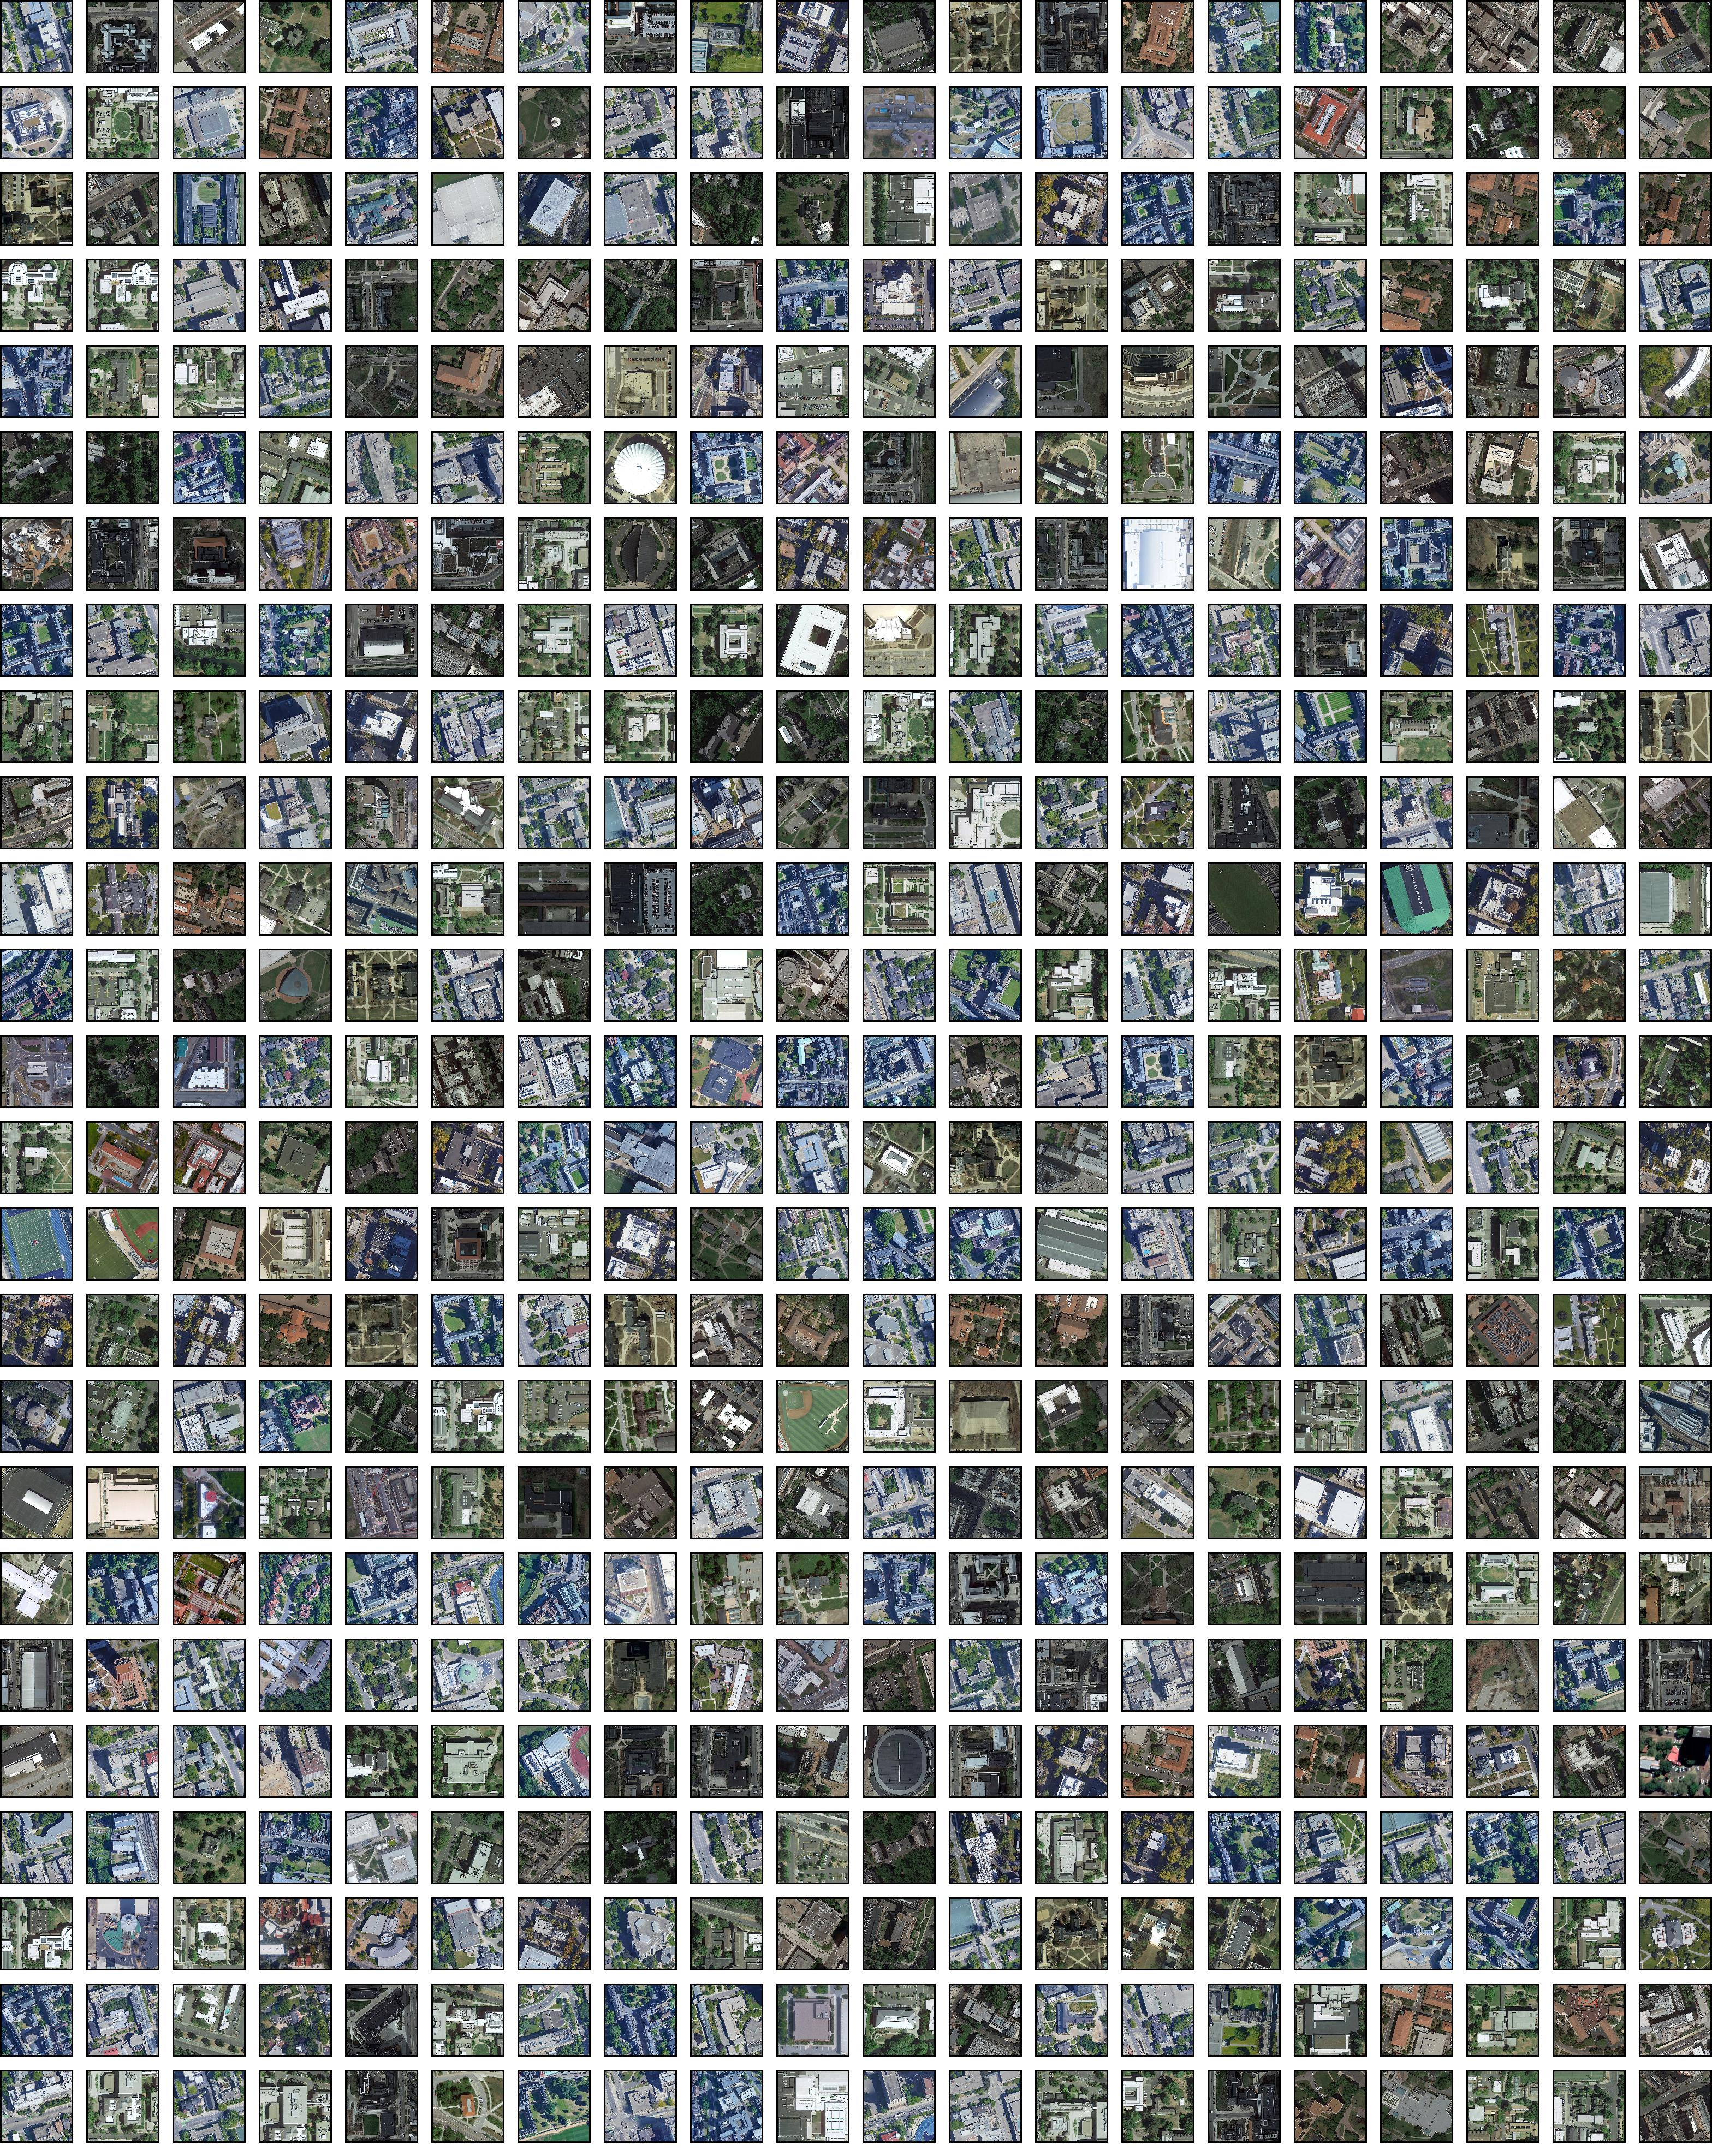}
\end{center}
%\vspace{-.25in}
     \caption{Images sampled from satellite-view images of the University-1652 dataset.
     }\label{fig:satellite-data}
\end{figure*}

\begin{figure*}[t]
\begin{center}
    \includegraphics[width=0.95\linewidth]{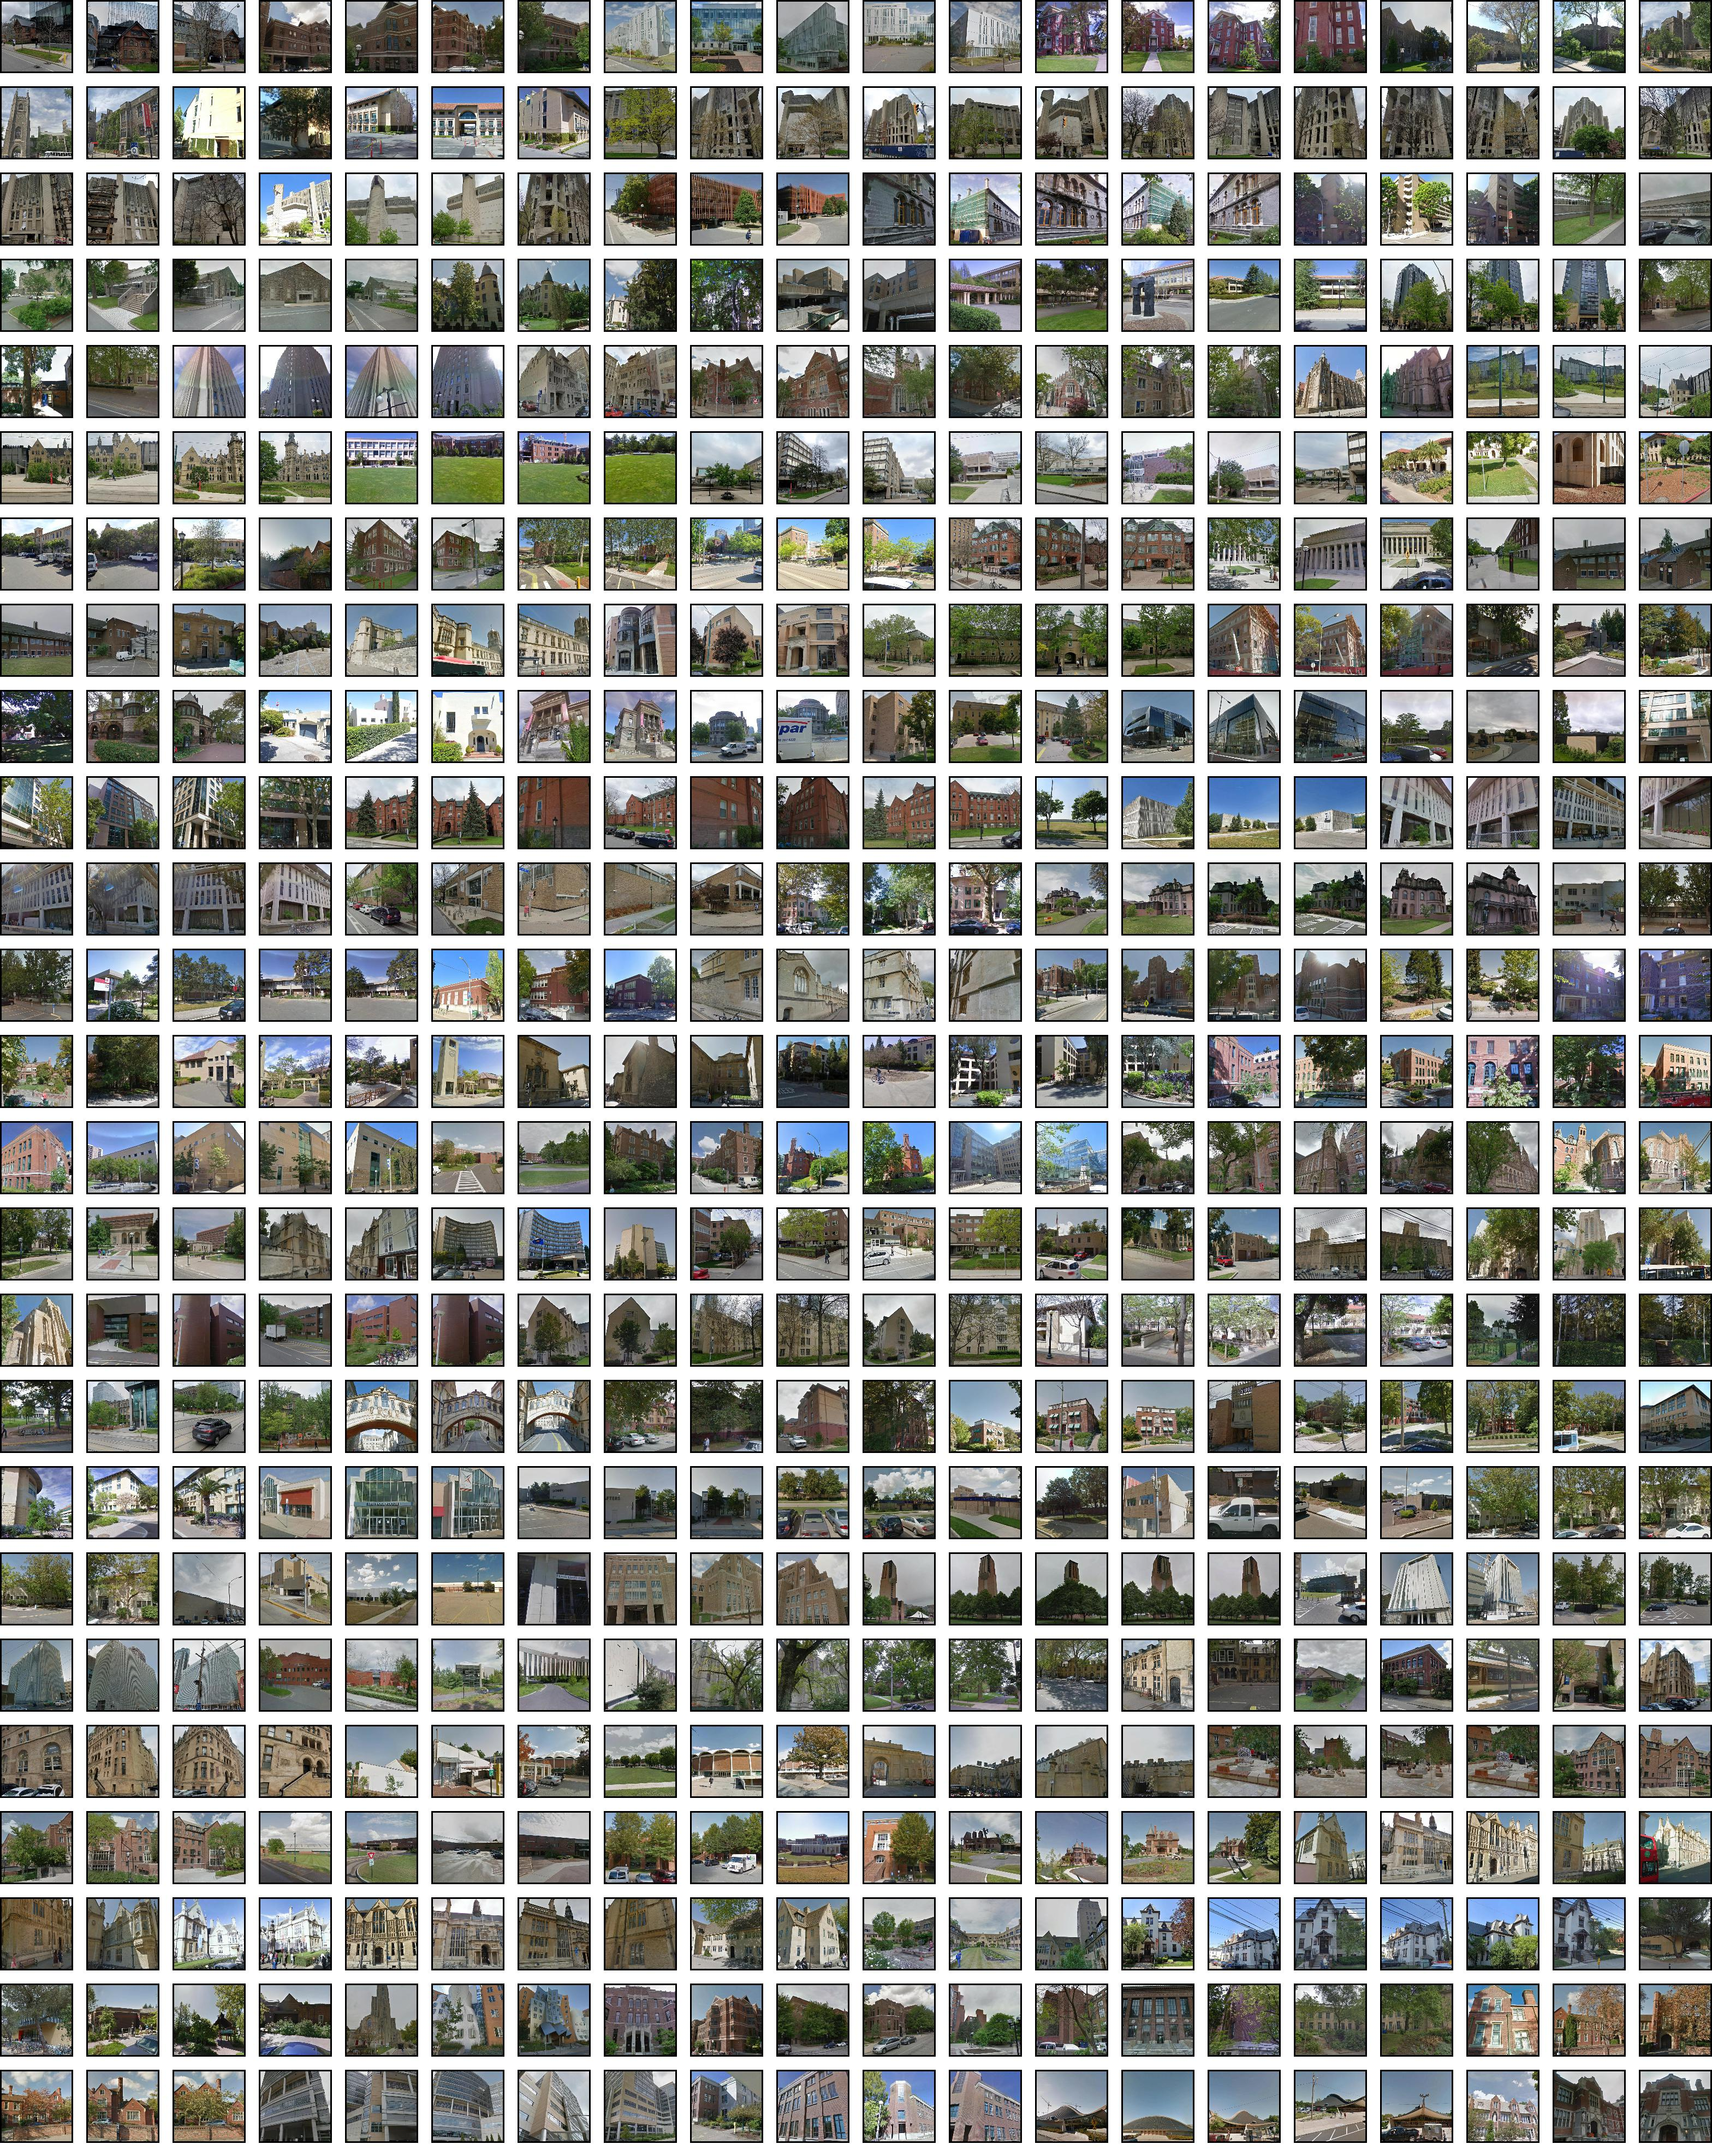}
\end{center}
%\vspace{-.25in}
     \caption{Images sampled from ground-view images of the University-1652 dataset (collected from Google Street View).
     }\label{fig:ground-data}
\end{figure*}

\begin{figure*}[t]
\begin{center}
    \includegraphics[width=0.95\linewidth]{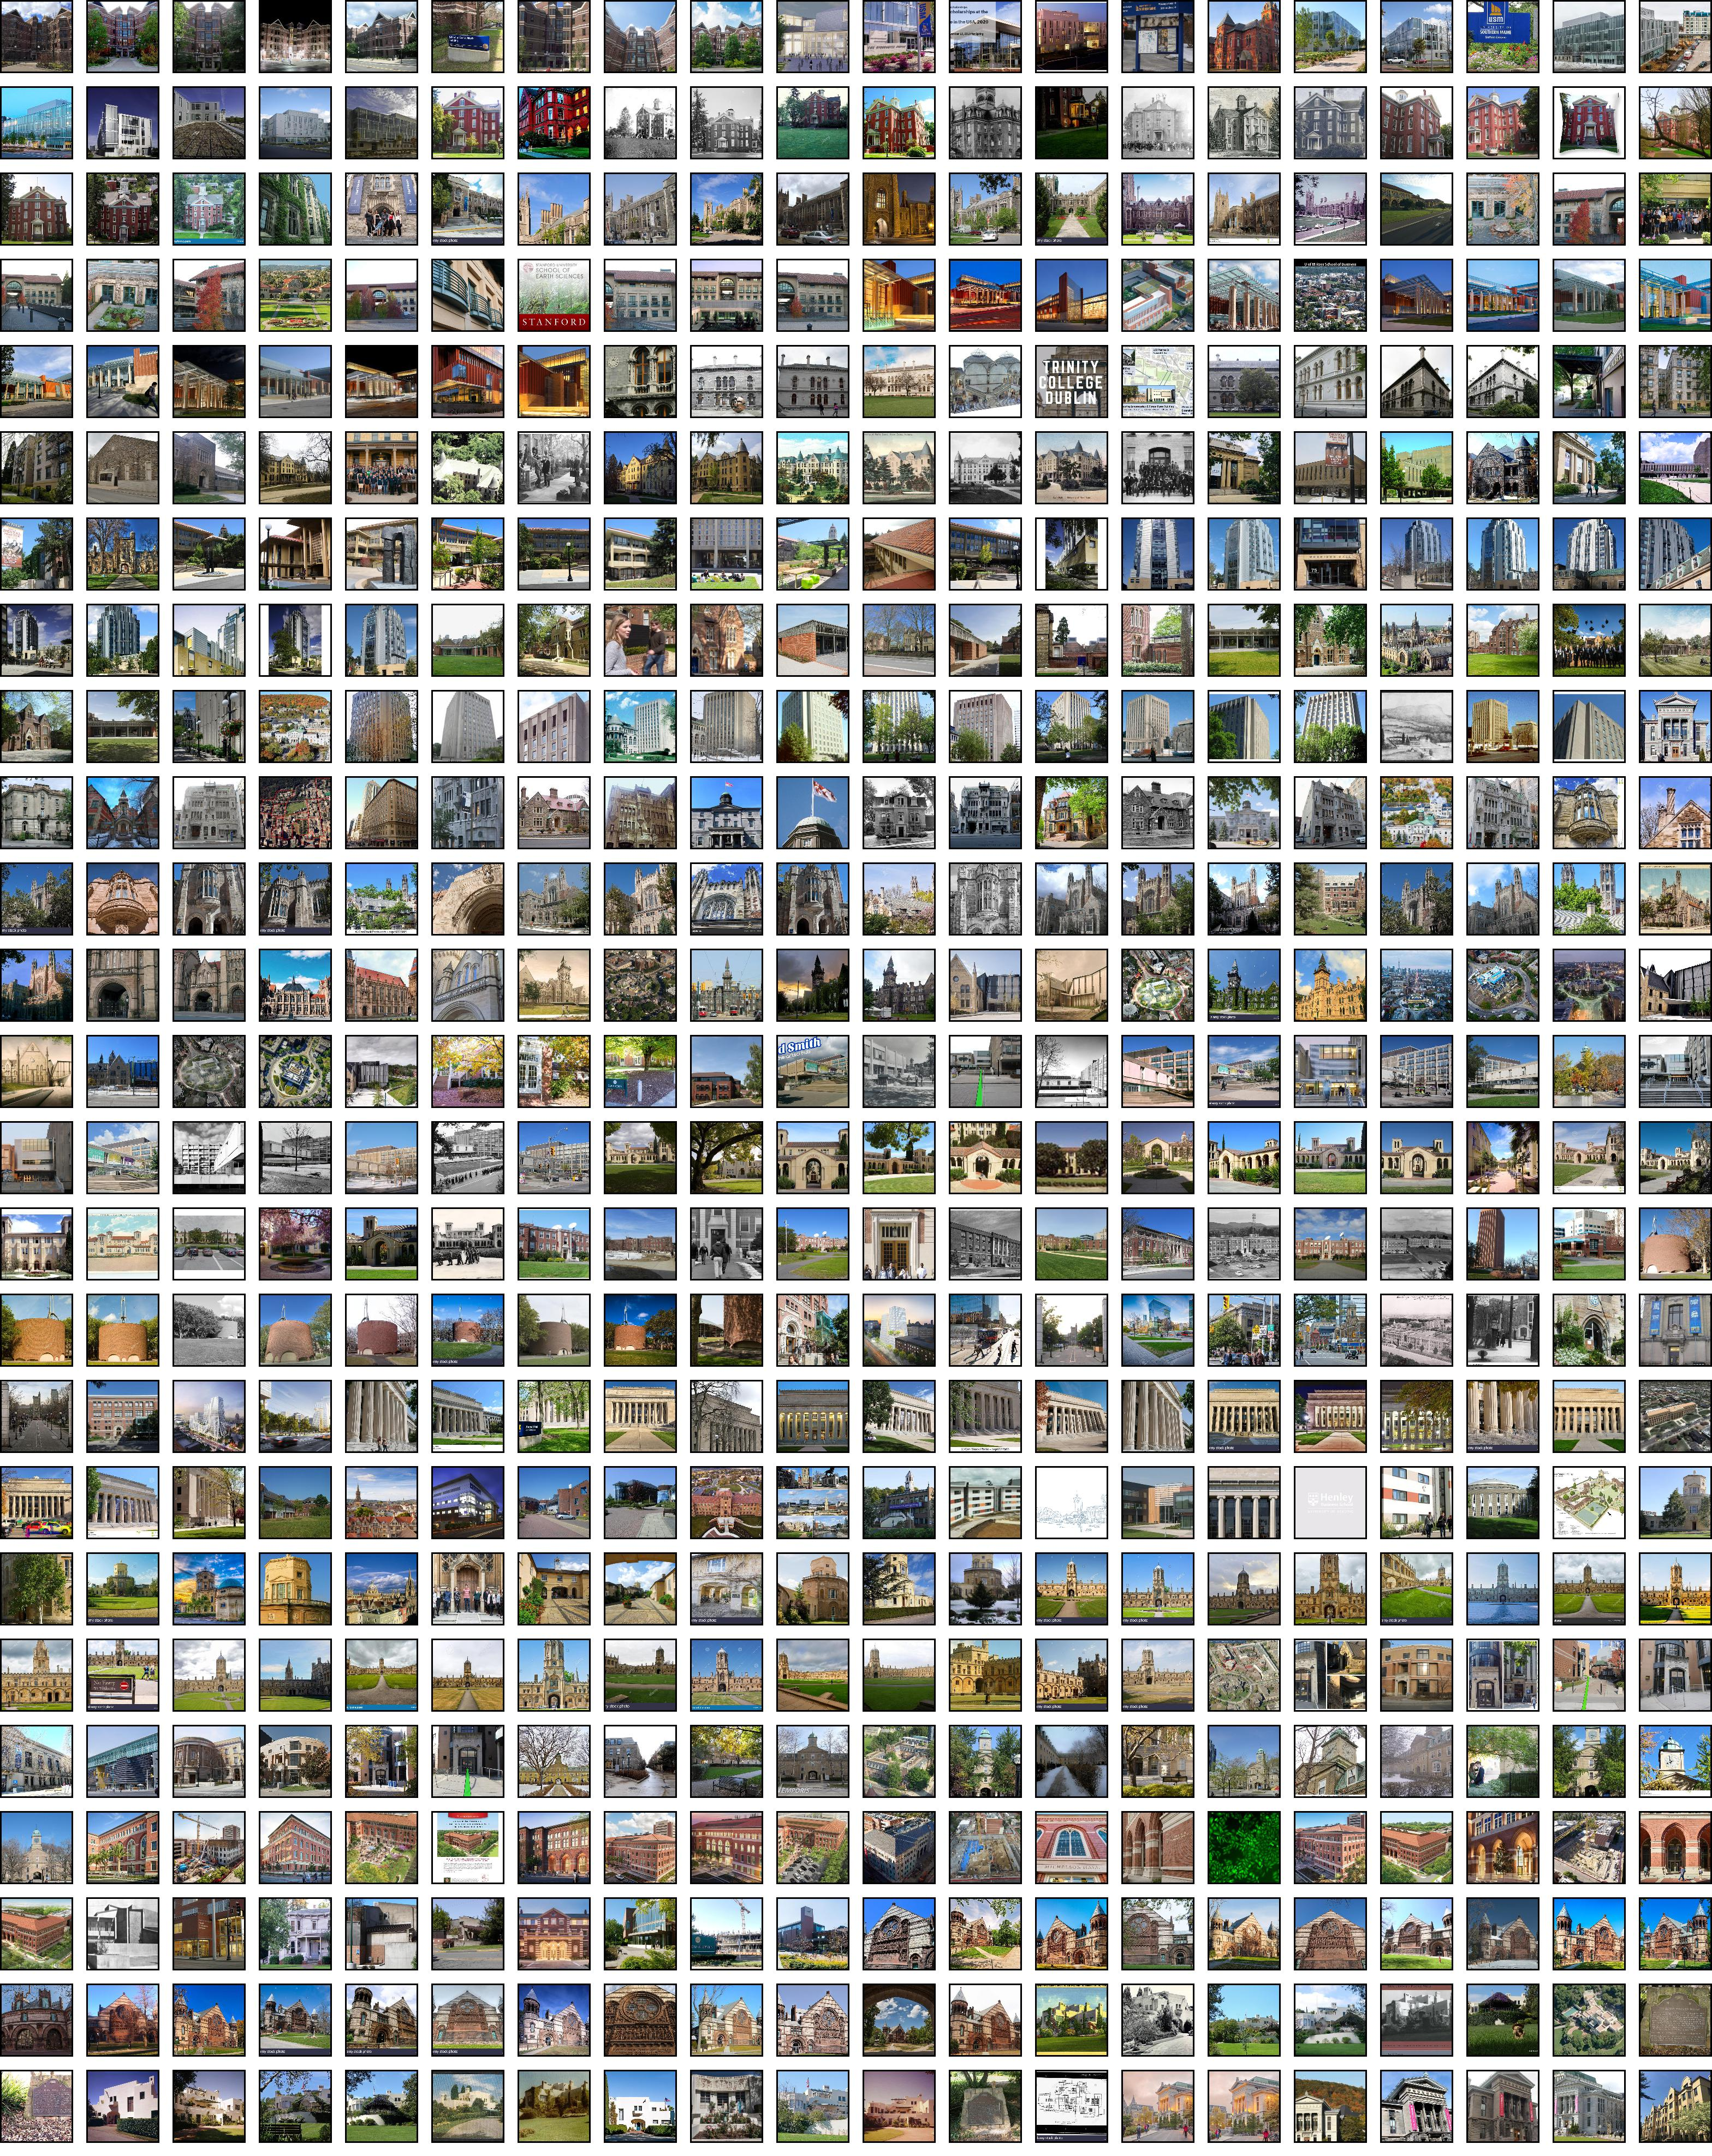}
\end{center}
%\vspace{-.25in}
     \caption{Images sampled from ground-view images (noisy) of the University-1652 dataset (collected from Google Image).
     }\label{fig:google-data}
\end{figure*}

\end{comment}
